# Supplementary material for: Computational Physics: An Introduction to Monte Carlo Simulations of Matrix Field Theory
Source: arXiv:1506.02567 source file (2016-03-15)
Supplement: Supplementary file 1 [file CP-MC-MFT-YDRI-Y-Appendix-B.pdf]

# اعمال تطبيقية في الفيزياء العددية

باديس يدري

معهد الفيزياء، جامعة باجي مختار، عنابة، الجزائر

جانفي 2015

# الفهرس


0 مقدمة . . . . . . . . . . . . . . . . . . . . . . . . . . . . . . . . . . . . 310
1 خوارزمية اولر- مقاومة الهواء . . . . . . . . . . . . . . . . . . . . . . . . . . . . 312
2 حركة القذائف تحت تأثير مقاومة الهواء . . . . . . . . . . . . . . . . . . . . . . . . 313
3 الهزاز التوافقي- خوارزميات اولر- كرومر و فيرلات . . . . . . . . . . . . . . . . . . . 314
4 التكاملات العددية . . . . . . . . . . . . . . . . . . . . . . . . . . . . . . . . 316
5 خوارزميات نيوتن - رافسون . . . . . . . . . . . . . . . . . . . . . . . . . . . . 317
6 خوارزمية رونج - كوتا- المجموعة الشمسية . . . . . . . . . . . . . . . . . . . . . . 318
7 مسألة دوران الحضيض الشمسي لكوكب عطارد . . . . . . . . . . . . . . . . . . . . . 320
8 النواس الفوضوي 1 : تأثير الفراشة . . . . . . . . . . . . . . . . . . . . . . . . . 322
9 النواس الفوضوي 2 : مقاطع بوانكري . . . . . . . . . . . . . . . . . . . . . . . . 324
10 النواس الفوضوي 3 : ظاهرة تضاعف الدور . . . . . . . . . . . . . . . . . . . . . . 326
11 النواس الفوضوي 4: مخططات الانشطار و الانكسار التلقائي للتناظر . . . . . . . . . . 327
12 الديناميك الجزيئي 1: توزيع ماكسويل . . . . . . . . . . . . . . . . . . . . . . . . 330
13 الديناميك الجزيئي 2: الانصهار . . . . . . . . . . . . . . . . . . . . . . . . . . 332
14 الاعداد العشوائية . . . . . . . . . . . . . . . . . . . . . . . . . . . . . . . . 333
15 المشاء العشوائي . . . . . . . . . . . . . . . . . . . . . . . . . . . . . . . . 334
16 تقريبات النقطة الوسطي و مونتي كارلو . . . . . . . . . . . . . . . . . . . . . . . 335
17 توزيعات الاحتمال غير المنتظمة . . . . . . . . . . . . . . . . . . . . . . . . . . 337
18 خوارزمية ميتروبوليس و نموذج ايزينغ . . . . . . . . . . . . . . . . . . . . . . . . 339
19 التغير الطوري من الرتبة الثانية الفيرومغناطيسي . . . . . . . . . . . . . . . . . . . 341
20 دالة الربط (غرين) الثنائية . . . . . . . . . . . . . . . . . . . . . . . . . . . . 342
21 الهستريسيس و التغير الطوري من الرتبة الاولي . . . . . . . . . . . . . . . . . . . . 344

# مقدمة

الفيزياء العددية هي احد فروع العلوم العددية التي تعرف ايضا باسم الحاسوبية العلمية و التي ظهرت و تبلورت خلال $40-30$ سنة الاخيرة مع التقدم الهائل الذي حصل في التكنولوجيا الرقمية خاصة في الولايات المتحدة الامريكية.

يمكن اعتبار الفيزياء العددية قسم من اقسام الفيزياء النظرية او يمكن اعتبارها جسر يربط بين الفيزياء النظرية و الفيزياء التجريبية و هناك حتي من يعتبرها تخصص قائم لخدمة الفيزياء التجريبية لا حسب. تقليديا هناك مقاربتان متكاملتان، علي الاقل منذ عصر نيوتن، للفيزياء. فهناك من ناحية المقاربة النظرية و من ناحية اخري هناك المقاربة التجريبية. هناك الكثير الان، خاصة من العاملين في هذا المجال و من غيرهم، من يعتبر انه توجد مقاربة ثالثة منفصلة و مختلفة للفيزياء هي المقاربة العددية. من وجهة النظر هذه فان الفيزياء العددية هي حقل منفصل بذاته غير مرتبط بالضرورة بالحقلين النظري و التجريبي. رغم هذا فان وجهة النظر التي سوف نتبناها في هذه المطوية هو الراي الاول الذي يعتبر ان الفيزياء العددية هو فرع من فروع الفيزياء النظرية.

في الفيزياء العددية يتم مزج عناصر من الفيزياء و خاصة الفيزياء النظرية و عناصر من الرياضيات التطبيقية مثل التحليل العددي مع عناصر من علوم الحاسوب مثل البرمجة من اجل هدف واحد هو حل مسالة فيزيائية معينة ليس لها حل كامل او حل معروف.

اهم استعمالات الكمبيوتر في الفيزياء هو اجراء المحاكيات (جمع محاكاة) العددية. المحاكيات العددية تلائم اكثر المسائل الفيزيائية التي تتحكم فيها معادلات رياضية غير خطية و التي لا تتوفر في معظمها علي حل تحليلي مضبوط. نقطة البدء لاي محاكاة عددية هو نموذج مثالي للجملة الفيزيائية قيد الدراسة و من الطبيعي اننا نريد ان نتأكد ما اذا كان تصرف هذا النموذج منسجم مع المشاهدة او لا في حالة توفر نتائج تجريبية للمقارنة اما في حالة عدم توفر اي نتائج تجريبية فان الهدف هو استشراف ما يمكن ان تعطيه التجربة اذا ما اجريت. الخطوة الاولي من اجل تحقيق هذا الهدف هو ايجاد خوارزمية رياضية من اجل انجاز هذا النموذج نظريا و ايضا علي الكمبيوتر. تنفيذ هذا الانجاز علي كمبيوتر هو ما نسميه بالمحاكاة العددية و هو يعتمد علي ترجمة الخوارزمية الرياضية الي شفرة مكتوبة باحدي لغات البرمجة يمكن للكمبيوتر ان يفهمها.

المحاكيات العددية هي اذن تجارب افتراضية. فمثلا يلعب النموذج الرياضي في المحاكاة العددية بالضبط دور العينة في التجربة المعملية اما الخوارزمية اوالشفرة التي تستعملها المحاكاة العددية فهي تقوم بدور جهاز القياس في التجربة المعملية. قبل البدء في استعمال المحاكاة العددية في الدراسة الفيزيائية فانه علينا اختبار او معايرة الشفرة تماما كما اننا نقوم بمعايرة جهاز القياس في التجربة المعملية قبل البدء في اجراء اي قياس. القياس الذي نقوم به في التجرية المعملية يقابله الحساب الذي تجريه المحاكاة العددية و نختتم كلا العمليتين بنفس الأمر و هو تحليل المعطيات.

من الواضح جدا و من الطبيعي ان اهم وسائل الفيزياء العددية هي لغات البرمجة. في معظم المحاكيات العددية التي نجدها في الاعمال البحثية الفيزيائية تكتب الشفرات في احدي اللغات المجمعة مثل الفرترون (Fortran) او لغة سي ($C$). في هذه المحاكيات يمكن ايضا عند الحاجة مناداة مكتبات الروتينات العددية مثل لاباك (Lapack) و غيرها. استعمال البرمجيات العددية الجاهزة مثل ماتلاب (Matlab) و ماثيماتيكا (Mathematica) في هذه المحاكيات العددية، خاصة التي تعتمد علي طريقة المونتي كارلو (Monte Carlo)، غير عملي بالمرة لانه يؤدي الي زمن

سير طويل جدا للشفرة علي الكمبيوتر و هذا راجع بالخصوص الي كون البرمجيات الجاهزة هي لغات مترجمة و ليست لغات مجمعة. ليس هناك ادني شك في ان البرمجيات الجاهزة مفيدة للغاية في الحسابات العددية التي لا تعتمد علي التكرار لكنها غير ملائمة تماما في المحاكيات العددية التي تعتمد بالاساس علي تكرار نفس الخطوة عدد هائل من المرات. في هذه المطوية سوف نتبع بالضبط هذا الطريق اي سوف نكتب جميع شفراتنا في لغة مجمعة و نتجنب استخدام البرمجيات الجاهزة. سوف نستخدم بالخصوص الفرترون 77 او 90 علي نظام التشغيل لينيكس (Linux) توزيع يوبنتو (Ubuntu) .

هذه المطوية تحتوي علي مجموع الاعمال التطبيقية المرفقة بمحاضرات الفيزياء العددية التي القاها المؤلف باديس ايدري في معهد الفيزياء منذ العام 2009 علي طلبة الليسانس و الماستر في اطار مقاييس التحليل العددي (ليسانس فيزياء)، الفيزياء العددية (ماستر فيزياء نظرية) و الاعلام الالي (باقي تخصصات الماستر). يمكن الحصول علي مطوية -محاضرات في الفيزياء العددية- عن طريق الاتصال بالمؤلف باديس ايدري عبر البريد الالكتروني badis.ydri@univ − annaba.org او تصفح الموقع الرسمي خاصته علي .http : //homepages.dias.ie/ydri/

في الختام يتقدم المؤلف باديس ايدري اصالة عن نفسه و عن باقي فريق العمل بالشكر الجزيل للمدير السابق لمعهد الفيزياء الاستاذ مصطفي بن شهاب و كذلك للمدير الحالي الاستاذ علاوة شيباني للمساعدات الجليلة و التسهيلات الكثيرة التي قدماها منذ البداية من اجل ادخال هذه المحاضرات و التطبيقات في البرامج الرسمية للفيزياء.

باديس يدري
سرايدي، عنابة، الجزائر
الاثنين 8 جويلية 2013

# خوارزمية اولر- مقاومة الهواء

يقود رياضي دراجة هوائية علي طريق مستقيمة و مسطحة بسرعة $v$ . القوة التي يطبقها الرياضي علي الدراجة تكافئ استطاعة ثابتة $P$ تساوي $200$ واط يوفرها الرياضي لفترة زمنية تقدر بساعة واحدة. قوة مقاومة الهواء (التي تعرف ايضا بقوة الجر الهوائي) تكون معاكسة للحركة و متناسبة طردا مع مربع السرعة معطاة بالعلاقة

$$F_{\rm drag} = -C\rho A v^2.$$

في هذه المعادلة $\rho$ هي كثافة الهواء، $C$ هو معامل الجر و $A$ هي مساحة المقطع العرضي لجملة الرياضي زائد الدراجة. قانون نيوتن الثاني يأخذ الشكل التالي

$$\frac{dv}{dt} = \frac{P}{mv} - \frac{C\rho A v^2}{m}.$$

المطلوب هو حساب السرعة $v$ كدالة في الزمن. المقاربة العددية لهذه المسألة تعتمد علي خوارزمية اولر. نقطع المجال الزمني $T$ الي $N$ مجال زمني صغير

$$\Delta t = \frac{T}{N}$$

اي

$$t = i\Delta t \ , \ i = 0, ..., N.$$

نعرف

$$\hat{v}(i) = v(t - \Delta t).$$

الحل المعطي بتقريب اولر يأخذ الشكل

$$\hat{v}(i+1) = \hat{v}(i) + \Delta t\bigg(\frac{P}{m\hat{v}(i)} - \frac{C\rho A \hat{v}^2(i)}{m}\bigg) \ . \ i = 1, ..., N+1$$

اللحظات الزمنية المرافقة تعطي ب

$$\hat{t}(i+1) = i\Delta t \ , \ i = 1, ..., N+1.$$

(1) احسب السرعة كدالة في الزمن في حالة وجود مقاومة الهواء وفي حالة عدم وجود مقاومة الهواء. ماذا تلاحظ. في هذا السؤال نأخذ ثابت الجر $C$ يساوي $0.5$. نعطي ايضا القيم

$$m = 70{\rm kg} \ , \ A = 0.33m^2 \ , \ \rho = 1.2{\rm kg}/m^3 \ , \ \Delta t = 0.1s \ , \ T = 200s.$$

السرعة الابتدائية تعطي ب

$$\hat{v}(1) = 4m/s \ , \ \hat{t}(1) = 0.$$

(2) ماذا تلاحظ في حالة تغيير ثابت الجر و/او الاستطاعة. ماذا تلاحظ عندما يتم تصغير الخطوة الزمنية.

# حركة القذائف تحت تأثير مقاومة الهواء

نعتبر حركة قذيفة تحت تأثير قوة مقاومة الهواء التي تعمل عكس اتجاه الحركة و تكون متناسبة مع مربع السرعة. نرمز لثابت التناسب ب $B$. قانون نيوتن الثاني يؤدي الي معادلات الحركة التالية

$$\frac{dx}{dt} = v_x \ , \ m\frac{dv_x}{dt} = -Bvv_x.$$

$$\frac{dy}{dt} = v_y \ , \ m\frac{dv_y}{dt} = -mg - Bvv_y.$$

حل هذه المعادلات التفاضلية المعطي بخوارزمية اولر بأخذ الشكل التالي

$$v_x(i+1) = v_x(i) - \Delta t\frac{Bv(i)v_x(i)}{m}.$$

$$v_y(i+1) = v_y(i) - \Delta tg - \Delta t\frac{Bv(i)v_y(i)}{m}.$$

$$v(i+1) = \sqrt{v_x^2(i+1) + v_y^2(i+1)}.$$

$$x(i+1) = x(i) + \Delta t \ v_x(i).$$

$$y(i+1) = y(i) + \Delta t \ v_y(i).$$

القيم الابتدائية للموضع و السرعة توافق القيمة $1$ ل $i$ و $i$ يأخذ القيم من $1$ الي $N$.

(1) اكتب شفرة فورترون منجز فيها الحل المعطي بخوارزمية اولر لمسألة.

(2) نأخذ القيم التالية

$$\frac{B}{m} = 0.00004m^{-1} \ , \ g = 9.8m/s^2.$$

$$v(1) = 700m/s \ , \ \theta = 30 \text{ degree}.$$

$$v_x(1) = v(1)\cos\theta \ , \ v_y(1) = v(1)\sin\theta.$$

$$N = 10^5 \ , \ \Delta t = 0.01s.$$

احسب المسار بدون و ب مقاومة الهواء. ماذا تلاحظ.

(3) باستخدام التصريح الشرطي $if$ يمكن تعيين مدي القذيفة. هذا التصريح يضاف داخل حلقة $do$ كالتالي

$$\text{if}(y(i+1).\text{le}.0)\text{exit}.$$

عين مدي القذيفة في حالة وجود و في حالة عدم وجود مقاومة للهواء.

(4) في حالة عدم وجود مقاومة للهواء نعرف ان المدي يأخذ اعظم قيمة له لما تكون الزاوية الابتدائية تساوي $45$ درجة. تحقق من هذا الامر عدديا باختبار عدة قيم للزاوية الابتدائية. يمكن ايضا اضافة حلقة $do$ في الزاوية ثم دراسة المدي كدالة في الزاوية و البحث عن قيمته العظمي.

(5) في حالة وجود مقاومة الهواء احسب الزاوية التي يكون فيها المدي اعظمي.

# الهزاز التوافقي- خوارزميات اولر- كرومر و فيرلات

نعتبر هزاز توافقي بسيط عبارة عن كتلة $m$ مربوطة بخيط طوله $l$ معلق في مرتكز ثابت تحت تأثير الثقالة $g$. نفترض ان الحركة خطية اي ان الزاوية التي يصنعها النواس مع المحور الشاقولي تبقي دائما صغيره. معادلة الاهتزاز المشتقة من قانون نيوتن الثاني تأخذ الشكل

$$\frac{d^2\theta}{dt^2} + \frac{g}{l}\theta = 0.$$

هذه المعادلة التفاضلية من الرتبه الثانيه يمكن تعويضها بمعادلتين تفاضليتين من الرتبة الاولي كالتالي

$$\frac{d\theta}{dt} = \Omega \ , \ \frac{d\Omega}{dt} = -\frac{g}{l}\theta.$$

الحل العددي الاول الذي سنعتبره هنا هو الحل المعطي بخوارزمية اولر

$$\Omega_{i+1} = \Omega_i - \frac{g}{l}\theta_i \ \Delta t.$$

$$\theta_{i+1} = \theta_i + \Omega_i \ \Delta t.$$

الحل العددي الاخر الذي سنعتبره هنا هو الحل المعطي بخوارزمية اولر- كرومر. هذا الحل يعطي بالمعادلات التالية

$$\Omega_{i+1} = \Omega_i - \frac{g}{l}\theta_i \ \Delta t.$$

$$\theta_{i+1} = \theta_i + \Omega_{i+1} \ \Delta t.$$

نعتبر هنا ايضا الحل المعطي بخوارزمية فيرلات الذي يأخذ الشكل

$$\theta_{i+1} = 2\theta_i - \theta_{i-1} - \frac{g}{l}\theta_i(\Delta t)^2.$$

(1) اكتب شفرة فورترون منجز فيها الحلول المعطاة بخوارزميات اولر و اولر- كرومر لمسألة الهزاز التوافقي.

(2) احسب الزاوية، السرعة الزاوية و الطاقة كدوال في الزمن. طاقة الهزاز تعطي ب

$$E = \frac{1}{2}\Omega^2 + \frac{1}{2}\frac{g}{l}\theta^2.$$

نأخذ القيم العددية

$$g = 9.8m/s^2 \ , l = 1m \ .$$

نأخذ عدد الخطوات و الخطوة الزمنية

$$N = 10000 \ , \ \Delta t = 0.05s.$$

نأخذ الزاوية و السرعة الزاوية الابتدائيتان

$$\theta_1 = 0.1\text{radian} \ , \ \Omega_1 = 0.$$

باستعمال التصريح الشرطي $if$ يمكن تحديد زمن الحركة بخمسة اضعاف الدور كالتالي

$$\text{if}(t(i+1).\text{ge}.5 * \text{period}) \text{ exit}.$$

(3) قارن بين قيمة الطاقة المحسوبة باولر و قيمة الطاقة المحسوبة باولر- كرومر. ماذا تلاحظ و ماذا تستنتج.

(4) اعد الحساب باستخدام خوارزمية فيرلات. لنلاحظ ان هذه الطريقة لا يمكنها الانطلاق فقط من القيم الابتدائية $\theta_1$ و $\Omega_1$. يجب ايضا اعطاء الزاوية $\theta_2$ التي يمكن حسابها باستعمال طريقة اولر اي

$$\theta_2 = \theta_1 + \Omega_1 \, \Delta t.$$

لنلاحظ ايضا ان خوارزمية فيرلات لا تحتاج الي حساب السرعة الزاوية. لكن من اجل حساب الطاقة نحتاج الي معرفة السرعة الزاوية التي نحسبها باستعمال العبارة

$$\Omega_i = \frac{\theta_{i+1} - \theta_{i-1}}{2\Delta t}.$$

# التكاملات العددية

نعتبر التكاملات في بعد واحد من الشكل

$$I = \int_a^b dx f(x).$$

نعتبر الحالة العامة التي لا يمكن فيها اجراء التكامل تحليليا و يبقي الحل العددي هو الخيار الوحيد . الخوارزميات التي سنستعملها هي التقريب بالمستطيلات و بأشباه المنحرف و التقريب بقطوع المكافئ . في كل هذه الطرق نقسم مجال التعريف الي $N$ مجال طوله $\Delta x$ كالتالي

$$x_i = x_0 + i\Delta x \ , \ i = 0, ..., N \ , \ \Delta x = \frac{b-a}{N} \ , \ x_0 = a, x_N = b.$$

التقريب بالمستطيلات يعطي ب

$$F_N = \Delta x \sum_{i=0}^{N-1} f(x_i).$$

التقريب باشباه المنحرف يعطي ب

$$T_N = \Delta x \bigg[\frac{1}{2} f(x_0) + \sum_{i=1}^{N-1} f(x_i) + \frac{1}{2} f(x_N)\bigg].$$

التقريب بقطوع المكافئ (قاعدة سيمبسون) يعطي ب ( هنا $N$ يجب ان يكون زوجي)

$$S_N = \frac{\Delta x}{3} \bigg[f(x_0) + 4 \sum_{i=0}^{\frac{N-2}{2}} f(x_{2i+1}) + 2 \sum_{i=0}^{\frac{N-2}{2}} f(x_{2i}) + f(x_N)\bigg].$$

الخطأ في هذه التقريبات الثلاث متناسب مع $1/N$، $1/N^2$ و مع $1/N^4$ علي التوالي .

(1) نأخذ التكامل

$$I = \int_0^1 f(x) dx \ ; \ f(x) = 2x + 3x^2 + 4x^3.$$

احسب قيمة هذا التكامل باستعمال طريقة المستطيلات. قارن مع قيمة التكامل التحليلية.
ملاحظة: شفر الدالة باستعمال subroutine او function .

(2) غير عدد المجالات $N$ . احسب الخطأ المرتكب بدلالة $N$. قارن مع النظري.

(3) اعد السؤالين السابقين باستعمال طريقة اشباه المنحرف و قاعدة سيمبسون.

(4) خذ الان التكاملات التالية

$$I = \int_0^{\frac{\pi}{2}} \cos x dx \ , \quad I = \int_1^e \frac{1}{x} dx \ , \ I = \int_{-1}^{+1} \lim_{\epsilon \longrightarrow 0} \bigg(\frac{1}{\pi} \frac{\epsilon}{x^2 + \epsilon^2}\bigg) dx.$$

# خوارزمية نيوتن - رافسون

جسيم ذو كتلة $m$ يتحرك في بئر كمون ارتفاعه $V$ و طوله $2a$ يمتد من $-a$ الي $+a$. نهتم بحالات الجملة ذات الطاقات الاصغر من ارتفاع البئر اي الحالات المرتبطة. حالة الجملة قد تكون زوجية او فردية. الطاقات المسموح بها المرفقة بالدوال الموجية الزوجية تعطي بحلول المعادلة المتسامية

$$\alpha \tan \alpha a = \beta.$$

$$\alpha = \sqrt{\frac{2mE}{\hbar^2}}\ ,\ \beta = \sqrt{\frac{2m(V-E)}{\hbar^2}}.$$

في حالة بئر الكمون اللانهائي نجد الحلول

$$E_n = \frac{(n+\frac{1}{2})^2\pi^2\hbar^2}{2ma^2}\ ,\ n = 0, 1....$$

نختار(مع اهمال كتابة الوحدات)

$$\hbar = 1\ ,\ a = 1\ ,\ 2m = 1.$$

من اجل ايجاد الطاقات $E$ نستعمل خوارزمية نيوتن - رافسون التي تسمح لنا بايجاد جذور اي معادلة $f(x) = 0$ كالتالي. انطلاقا من تخمين معين $x_0$ فاننا نقرب حل المعادلة $f(x) = 0$ بنقطة تقاطع مماس الدالة $f(x)$ في النقطة $x_0$ مع محور السينات. نسمي هذا التقريب الاول $x_1$ و هو يعطي بالمعادلة

$$x_1 = x_0 - \frac{f(x_0)}{f'(x_0)}.$$

انطلاقا من $x_1$ نقوم بنفس الخطوة من اجل ايجاد التقريب الثاني $x_2$ ثم نستخدم $x_2$ من اجل ايجاد التقريب الثالث $x_3$ و هكذا. التقريب $x_{i+1}$ يعطي بدلالة التقريب $x_i$ بالعلاقة

$$x_{i+1} = x_i - \frac{f(x_i)}{f'(x_i)}.$$

(1) من اجل $V = 10$ بين عدد الحلول $E$ باستعمال الطريقة البيانية عبر دراسة الدالتين

$$f(\alpha) = \tan \alpha a\ ,\ g(\alpha) = \frac{\beta}{\alpha} = \sqrt{\frac{V}{\alpha^2} - 1}.$$

(2) جد باستعمال طريقة نيوتن-رافسون الحلين بدقة اقل او تساوي من $10^{-8}$. من اجل ايجاد الحل الاول نأخذ التخمين الاول لطريقة نيوتن-رافسون في نقطة التباعد الاولي لدالة الظل اي $\alpha = \pi/a$. من اجل ايجاد الحل الثاني نأخذ التخمين الاول في نقطة التباعد الثانية اي $\alpha = 2\pi/a$.

(3) اعد السؤال من اجل $V = 20$ .

(4) حدد الحلول الاربعة من اجل$V = 100$. استعن بالطريقة البيانية من اجل تحديد التخمين الاول كل مرة.

(5) اعد الاسئلة السابقة باستعمال طريقة التنصيف.

# خوارزمية رونج - كوتا- المجموعة الشمسية

نعتبر مجموعة شمسية مشكلة من كوكب واحد يتحرك حول الشمس. نفترض ان كتلة الشمس ثقيلة جدا بالمقارنة مع كتلة الكوكب بحيث يمكن اعتبارها ساكنة في مركز النظام. قانون نيوتن الثاني يعطي معادلات الحركة التالية

$$v_x = \frac{dx}{dt} \ , \ \frac{dv_x}{dt} = -\frac{GM_s}{r^3}x \ , \ v_y = \frac{dy}{dt} \ , \ \frac{dv_y}{dt} = -\frac{GM_s}{r^3}y.$$

$$r = \sqrt{x^2+y^2}.$$

نستخدم الوحدات الفلكية حيث

$$GM_s = 4\pi^2 AU^3/yr^2.$$

حل معادلات الحركة الانفة الذكر المعطي بخوارزمية رونج- كوتا يأخذ الشكل

$$k_1 = \Delta t \ v_x(i) \ , \ p_1 = \Delta t \ v_y(i).$$

$$r(i) = \sqrt{x(i)^2+y(i)^2}.$$

$$k_3 = -\frac{GM_s}{r(i)^3}x(i)\Delta t \ , \ p_3 = -\frac{GM_s}{r(i)^3}y(i)\Delta t.$$

$$k_2 = (v_x(i) + \frac{1}{2}k_3)\Delta t \ , \ p_2 = (v_y(i) + \frac{1}{2}p_3)\Delta t.$$

$$R(i) = \sqrt{(x(i)+\frac{1}{2}k_1)^2 + (y(i)+\frac{1}{2}p_1)^2}.$$

$$k_4 = -\frac{GM_s}{R(i)^3}(x(i)+\frac{1}{2}k_1)\Delta t \ , \ p_4 = -\frac{GM_s}{R(i)^3}(y(i)+\frac{1}{2}p_1)\Delta t.$$

$$x(i+1) = x(i) + k_2.$$

$$v_x(i+1) = v_x(i) + k_4.$$

$$y(i+1) = y(i) + p_2.$$

$$v_y(i+1) = v_y(i) + p_4.$$

في المعادلات السابقة $i$ يأخذ القيم من $1$ الي $N$ . القيم الابتدائية للموضع و السرعة توافق القيمة $1$ ل $i$.

(1) اكتب شفرة فورترون منجز فيها الحل المعطي بخوارزمية رونج - كوتا لمسألة النظام الشمسي.

(2) احسب المسار و السرعة و كذلك الطاقة كدوال في الزمن. ماذا تلاحظ بالنسبة للطاقة. استخدم الوحدات الفلكية. للتذكير فان طاقة الكوكب في وحدة الكتلة تعطي ب

$$E = \frac{1}{2}v^2 - \frac{GM_s}{r}.$$

(3) حسب قانون كبلر الاول فان جميع المدارات هي قطوع ناقصة مع وجود الشمس في احد المحرقين. في ما يلي سنعتبر فقط الكواكب التي نعلم من المشاهدة ان مداراتها دائرية الي حد كبير. هذه الكواكب هي الزهرة و الارض و المريخ و المشتري و ساتورن. انصاف الاقطار تعطي في وحدة الوحدات الفلكية ب

$$a_{\rm venus}=0.72\ ,\ a_{\rm earth}=1\ ,\ a_{\rm mars}=1.52\ ,\ a_{\rm jupiter}=5.2\ ,\ a_{\rm saturn}=9.54.$$

تحقق من قانون كبلر الاول من اجل كل هذه الكواكب.

من اجل الاجابة علي السؤالين السابقين 2 و 3 نأخذ الشروط الابتدائية

$$x(1)=a\ ,\ y(1)=0\ ,\ v_x(1)=0\ ,\ v_y(1)=v.$$

القيمة التي تأخذها السرعة الابتدائية مهمة جدا من اجل الحصول علي المسار الصحيح و يتم تعيينها مثلا من افتراض ان المسار هو فعلا دائري و بالتالي فان قوة الجذب الثقالي تكون متوازنة مع قوة الطرد المركزي. نحصل علي

$$v=\sqrt{\frac{GM_s}{a}}.$$

ايضاأخذ الخطوة الزمنية و عدد التكرارات كالاتي

$$\Delta t=0.01yr\ ,\ N=10^3-10^4.$$

(4) حسب قانون كبلر الثالث فان مربع الدور يكون متناسب طردا مع مكعب نصف القطر. من اجل المدارات الدائرية فان ثابث التناسب يساوي بالضبط واحد. تحقق من هذا الامر من اجل كل الكواكب المذكورة اعلاه. يتم قياس الدور مثلا بمراقبة متي يرجع الكوكب الي ابعد نقطة له عن الشمس.

(5) بتغيير السرعة الابتدائية بطريقة مناسبة فانه يمكن الحصول علي مدار قطع ناقص. جرب هذا الامر.

(6) القانونان الاساسيان الذان يحكمان حركة النظام الشمسي المبسط الذي اعتبرناه في هذا التمرين هو قانون نيوتن للجذب الثقالي بين الكتل من جهة و قانون نيوتن الثاني من جهةاخري.

قانون الجذب الثقالي ينص في اهم بنوده في ان القوة بين الشمس و الكوكب مركزية موجهة من الكوكب نحو الشمس و متناسبة عكسا مع مربع المسافة. نفترض في الاتي ان قوة الجذب الثقالي هي متناسبة عكسا مع اس اخر للمسافة مختلف عن اثنين. غير الشفرة من اجل اخذ هذا التصرف الجديد للقوة بعين الاعتبار. احسب المدارات من اجل اساسات بين ثلاثة و واحد. ماذا تلاحظ و ماذا تستنتج.

# مسألة دوران الحضيض الشمسي لكوكب عطارد

حسب قانون كبلر الاول فان مدارات جميع الكواكب السيارة و من ضمنها عطارد تعطي بقطوع ناقصة مع وجود الشمس في احد المحرقين . هذا القانون يمكن اشتقاقه من تطبيق قوانين نيوتن علي تفاعل الكواكب مع الشمس مع افتراض انه يمكننا اهمال تفاعل الكواكب نفسها فيما بينها . تأثير الكواكب علي بعضها البعض يؤدي الي ظاهرة دوران محاور القطوع الناقصة حول الشمس و بالتالي الي دوران الحضيض الشمسي حول الشمس الذي هو اقرب نقطة في مسار الكوكب من الشمس . هذا الدوران للحضيض الشمسي حول الشمس يحدث لجميع الكواكب لكن مشاهدته صعبة للغاية بسبب كون اغلب المدارات هي دائرية الي حد كبير . فقط بلوتو و عطارد لها مدارات قطوع ناقصة ذات لاتراكزية كبيرة. لكن بالنسبة لبلوتو فان سرعته المدارية المنخفضة لا تسمح بمشاهدة دوران حضيضه الشمسي. يبقي عطارد الذي يمكن قياس دوران حضيضه حول الشمس بدقة معتبرة. قام الفلكيون بقياس سرعة الدوران التالية

$$566 \text{ arcsecond/century}.$$

اي ان حضيض عطارد يصنع دورة كاملة حول الشمس كل 240000 سنة. من جهة اخري فانه بتطبيق قوانين نيوتن علي تفاعل كوكب عطارد مع الشمس مع اخذ بعين الاعتبار تأثير باقي الكواكب علي عطارد نحسب سرعة الدوران

$$523 \text{ arcsecond/century}.$$

الفرق هو

$$43 \text{ arcsecond/century}.$$

هذه الكمية لا يمكن تفسيرها الا من خلال النسبية العامة اي من خلال فهمنا للثقالة علي انها قوة يتوسطها انحناء الفضاء-زمن. القوه الناجمة عن انحناء الفضاء-زمن بسبب كتلة الشمس والتي يستشعرها عطارد اكثر من غيره من الكواكب يمكن تقريبها ب

$$F=\frac{GM_sM_m}{r^2}(1+\frac{\alpha}{r^2})\ ,\ \alpha=1.1.10^{-8}AU^2.$$

الهدف هو التحقق عدديا من ان هذه القوة تؤدي فعلا الي كمية دوران للحضيض الشمسي لعطارد تساوي 43 قوس ثانية في القرن.

(1) عدل شفرة الفورترون التي استخدمناها في التطبيق السابق من اجل الاخذ بعين الاعتبار القوة المذكورة اعلاه .

أختيار الشروط الابتدائية مهم للغاية . الشرط الابتدائي الاول هو موضع عطارد . نختار

$$x_0=(1+e)a\ ,\ y_0=0.$$

اي اننا نختار الكوكب في اللحظة الابتدائية في ابعد نقطة له عن الشمس. نصف القطر الكبير $a$ لعطارد هو 0.39 وحدة فلكية و لاتراكزية عطارد $e$ تساوي 0.206 . المسافة $ea$ هي بعد الشمس التي توجد في احد المحرقين عن مركز القطع الناقص . الشرط الابتدائي الثاني هو سرعة عطارد في اللحظة الابتدائية التي تعطي ب

$$v_{x0}=0\ ,\ v_{y0}=\sqrt{\frac{GM_s}{a}\frac{1-e}{1+e}}.$$

هذه السرعة يمكن حسابها من تطبيق قانوني انحفاظ العزم الحركي و انحفاظ الطاقة بين النقطة الابتدائية اعلاه و النقطة $(x = 0, y = b)$ حيث $b$ هو نضف القطر الصغير لعطارد اي
$$b = a\sqrt{1 - e^2}.$$

(2) لان قيمه $\alpha$ التي تعطيها النسبية العامة صغيره جدا فان كمية دوران الحضيض الشمسي لعطارد ضئيلة يصعب ملاحظتها في اي محاكاه عددية ذات وقت محدود. نختار قيمة اكبر بكثير ل $\alpha$ مثلا
$$\alpha = 0.0008AU^2.$$

نختار ايضا
$$N = 20000\ ,\ dt = 0.0001.$$

احسب المدار من اجل هذه القيم . احسب الزاوية $\theta$ التي يصنعها الشعاع الذي يربط عطارد و الشمس مع المحور الافقي بدلالة الزمن . احسب ايضا المسافة بين الشمس و عطارد و مشتقتها بالنسبة للزمن اي
$$\frac{dr}{dt} = \frac{xv_x + yv_y}{r}.$$

هذه المشتقة تغير اشارتها كلما بلغ عطارد ابعد نقطة له عن الشمس او بلغ اقرب نقطة له (اي الحضيض الشمسي) عن الشمس . استخدم هذه الملاحظة من اجل رسم الزاوية $\theta_p$ لما يكون عطارد في ابعد نقطة له عن الشمس بدلالة الزمن . ماذا تلاحظ .

عين الميل $d\theta_p/dt$ الذي هو بالضبط كمية دوران الحضيض الشمسي لعطارد حول الشمس من اجل قيمة $\alpha$ المختارة اعلاه .

(3) اعد السؤال السابق من اجل قيم اخري ل $\alpha$ . نقترح
$$\alpha = 0.001, 0.002, 0.004.$$

في كل مرة احسب $d\theta_p/dt$ . ارسم $d\theta_p/dt$ بدلالة $\alpha$ . ماذا تلاحظ . اوجد الميل . استنتج كمية دوران الحضيض الشمسي لعطارد من اجل القيمة
$$\alpha = 1.1.10^{-8}AU^2.$$

(4) باستخدام معطيات السؤال السابق اوجد الدالة
$$\frac{d\theta_p}{dt} = f(\alpha).$$

باستعمال طريقة المربعات الاصغرية .

# النواس الفوضوي 1 : تأثير الفراشة

نواس عبارة عن كتلة $m$ مربوطة بخيط طوله $l$ معلق في مرتكز ثابت تحت تأثير الثقالة $g$ . حركة اي نواس هي حركة غير خطية عموما لان الزاوية التي يصنعها النواس مع المحور الشاقولي ليست بالضرورة صغيرة ويمكن ان تبلغ القيمة العظمي $\pi$ او القيمة الصغري $-\pi$ و بالتالي فان النواس يمكن ان يدور دورة كاملة تساوي 360 درجة حول نقطة ارتكازه. نأخذ بعين الاعتبار تأثير قوة مقاومة الهواء علي الكتلة $m$ ونفترض انها تعطي بقانون ستوكس الذي ينص علي ان مقاومة الهواء تكون معاكسه للحركة و متناسبة خطيا مع السرعة $d\theta/dt$ مع ثابت تناسب يساوي $mlq$:

$$F_{\rm drag}=-mlq\frac{d\theta}{dt}.$$

الاحتكاك مع الهواء يؤدي الي تخامد حركة النواس و توقفه عن الحركةبعد استهلاك النواس لكامل طاقته الابتدائية . من اجل الحفاظ علي حركة النواس ضد مقاومة الهواء من الضروري اضافة قوة تحريك خارجية التي نفترض انها قوة دورية في الزمن ذات تواتر $\nu_D$ و سعة ثابتة $mlF_D$ :

$$F_{\rm drive}=mlF_D\sin 2\pi\nu_D t.$$

معادلة الاهتزاز المشتقة من قانون نيوتن الثاني تأخذ الشكل

$$\frac{d^2\theta}{dt^2}=-\frac{g}{l}\sin\theta-q\frac{d\theta}{dt}+F_D\sin 2\pi\nu_D t.$$

نأخذ دائما التواتر الزاوي $\sqrt{g/l}$ المرفق بالاهتزازات البسيطة للنواس يساوي واحد اي $g=l$ .
الحل العددي الذي سنعتبره هنا هو الحل المعطي بخوارزمية اولر - كرومر:

$$\Omega_{i+1}=\Omega_i+\bigg(-\frac{g}{l}\sin\theta_i-q\Omega_i+F_D\sin 2\pi\nu_D t_i\bigg)\,\Delta t~,~\theta_{i+1}=\theta_i+\Omega_{i+1}\,\Delta t.$$

هذه الجملة الديناميكية تعرف باسم النواس الفوضوي (chaotic pendulum) و من اهم ما تتميز به الحساسية المفرطة للشروط الابتدائية . هذه الخاصية تعرف ايضا باسم تأثير الفراشة (butterfly effect) .

يمكن للهزازالفوضوي ان يتصرف بطريقتين مختلفتين . في المنطقة الخطية للهزاز الفوضوي الحركة دورية ذات دور يساوي دور قوة التحريك الخارجية اذا اهملنا الحركة الابتدائية العابرة . في المنطقة الفوضوية الحركة غير دورية لا تكرر نفسها ابدا و بالاضافة الي ذلك فان اي خطأ مهما كان متناه في الصغر في تحديد الشروط الابتدائية يؤدي الي حركة مختلفة بالكامل .

(1) اكتب شفرة منجز فيها الحل المعطي بخوارزمية اولر- كرومر لمسألة الهزاز الفوضوي . لنلاحظ ان الزاوية $\theta$ يمكن دائما اخذها محصورة في المجال $[-\pi,\pi]$ و في الحالة التي تكون فيها خارج هذا المجال نقوم باضافة $\pm 2\pi$ من اجل اعادة حصرها في المجال و هذا كالتالي

$$\text{if}(\theta_i.\text{lt.}\mp\pi)~\theta_i=\theta_i\pm 2\pi.$$

(2) نأخذ القيم و الشروط الابتدائية

$$dt = 0.04s\ ,\ 2\pi\nu_D = \frac{2}{3}s^{-1}\ ,\ q = \frac{1}{2}s^{-1}\ ,\ N = 1000 - 2000.$$

$$\theta_1 = 0.2 \text{ radian}\ ,\ \Omega_1 = 0 \text{ radian}/s.$$

$$F_D = 0 \text{ radian}/s^2\ ,\ F_D = 0.1 \text{ radian}/s^2\ ,\ F_D = 1.2 \text{ radian}/s^2.$$

ارسم الزاوية $\theta$ بدلالة الزمن. ماذا تلاحظ بالنسبة للقيمة الاولي لقوة التحريك الخارجية، ماهو تواتر الاهتزاز. ماذا تلاحظ بالنسبة للقيمة الثانية لقوة التحريك الخارجية، ماهو تواتر الاهتزاز من اجل الازمنة الصغري و ماهو تواتر الاهتزاز من اجل باقي الازمنة. ماذا تلاحظ بالنسبة للقيمة الثالثة . هل الحركة دورية .

# النواس الفوضوي 2 : مقاطع بوانكري

الحركة في المنطقة الفوضوية هي حركة حتمية لان تصرف الهزاز في جميع الازمنة اللاحقة يحسب من حل معادلة الحركة اعلاه مع اعطاء شروط ابتدائية ملائمة لكن لا يمكن التنبؤ بها. لكن هذا لا يعني ان الهزاز الفوضوي هو جملة عشوائية و هي خاصية يمكن رؤيتها بوضوح في مقاطع بوانكري .
عوض رسم المدار من اجل كل الازمنة يمكن ان نرسم فقط النقاط $(\theta, \Omega)$ في فضاء الطور من اجل الازمنة التي تحقق الشرط $\nu_D t = n$ . مجموعة النقاط التي نحصل عليها بهذه الطريقة تسمي مقطع بوانكري .
في المنطقة الخطية للهزاز الفوضوي تتكون حركة الهزاز من حركة ابتدائية عابرة في الازمنة الصغري و حركة دورية في باقي الازمنة . الجزء الدوري لا يتعلق بالشروط الابتدائية و لذلك يسمي المدار في فضاء الطور بالجاذب الدوري للهزاز الفوضوي . يتكون مقطع بوانكري من نقطة واحدة اذا اهملنا الحركة الابتدائية العابرة للهزاز الفوضوي و من الواضح ان هذا المقطع هو جاذب لانه لا يتعلق بالشروط الابتدائية .
مقطع بوانكري في المنطقة الفوضوية هو ايضا جاذب في فضاء الطور اي مدار لا يتعلق بالشروط الابتدائية يسمي بالجاذب الغريب مما يؤكد حقيقة ان الهزاز الفوضوي رغم انه جملة حتمية لا يمكن التنبؤ بتصرفها في المنطقة الفوضوية الا انه ليس بجملة عشوائية .

(1) نعتبر الان هزازان فوضويان $A$ و $B$ متماثلان في كل شئ لكن شروطهما الابتدائية مختلفة اختلافا طفيفا . مثلا نأخذ

$$\theta_1^A = 0.2 \text{ radian} \ , \ \theta_1^B = 0.201 \text{ radian}.$$

يقاس الاختلاف بين الحركتين $A$ و $B$ بالفرق بين الزاويتين $\theta_A$ و $\theta_B$:

$$\Delta\theta_i = \theta_i^A - \theta_i^B.$$

احسب $\ln \Delta\theta$ بدلالة الزمن من اجل

$$F_D = 0.1 \text{ radian}/s^2 \ , \ F_D = 1.2 \text{ radian}/s^2.$$

ماذا تلاحظ . هل الحركتان $A$ و $B$ متماثلتان . ماذا يحدث في الازمنة الكبري . هل حركة الهزاز الفوضوي هي من النوع الذي يمكن التنبؤ به . بالنسبة للقيمة الثانية استعمل

$$N = 10000 \ , \ dt = 0.01s.$$

(2) احسب السرعة الزاوية $\Omega$ بدلالة الزاوية $\theta$ من اجل

$$F_D = 0.5 \text{ radian}/s^2 \ , \ F_D = 1.2 \text{ radian}/s^2.$$

ماهو المدار في فضاء الطور من اجل الازمنة الصغري و ماذا يمثل. كيف يصبح المدار في الازمنة الكبري . قارن بين الهزازين $A$ و $B$ . هل يتعلق المدار في الازمنة الكبري بالشروط الابتدائية .

(3) للحصول علي مقطع بوانكري عدديا نرسم النقاط $(\theta, \Omega)$ في الازمنة التي تنعدم فيها الدالة $\sin \pi\nu_D t$ اي في الازمنة التي تغير فيها هذه الدالةاشارتها:

$$\text{if}(\sin \pi\nu_D t_i \sin \pi\nu_D t_{i+1}.\text{lt}.0)\text{then}$$

$$\text{write}(*,*)t_i, \theta_i, \Omega_i.$$

تحقق من ان مقطع بوانكري في المنطقة الخطية هو معطي بنقطة وحيدة في فضاء الطور . خذ مثلا

$$F_D = 0.5 \text{ radian}/s^2.$$

و استعمل

$$N = 10^4 - 10^7 \ , \ dt = 0.001s.$$

تحقق من ان مقطع بوانكري في المنطقة الفوضوية هو ايضا جاذب . خذ مثلا

$$F_D = 1.2 \text{ radian}/s^2.$$

و استعمل

$$N = 10^5 \ , \ dt = 0.04s.$$

قارن بين مقطع بوانكري للهزاز $A$ و مقطع بوانكري للهزاز $B$ . ماذا تلاحظ و ماذا تستنتج .

# النواس الفوضوي 3 : ظاهرة تضاعف الدور

من اهم الخصائص الفوضوية التي يتميز بها النواس الفوضوي هو ظاهرة تضاعف الدور. المدارات الدورية التي لها نفس دور قوة التحريك الخارجية تسمي الحركة ذات الدور واحد (period-1 motion) . لكن توجد ايضا مدارات ذات دور يساوي ضعف دور القوة الخارجية و مدارات ذات دور يساوي اربعة اضعاف دور القوة الخارجية و بصفة عامة مدارات ذات دور يساوي $2^{\mathcal{N}}$ ضعف دور القوة الخارجية . المدارات التي دورها يساوي $2^{\mathcal{N}}$ ضعف دور قوة التحريك الخارجية تسمي الحركة ذات الدور $\mathcal{N}$ (period-$\mathcal{N}$ motion) . في عالم الاهتزازات و الامواج المدارات التي نحصل عليها في العادة هي مدارات دورية ذات ادوار تساوي دور قوة التحريك الخارجية تقسيم $2^{\mathcal{N}}$ و هي ظاهرة تعرف باسم المزج (mixing). اذن ظاهرة تضاعف الدور التي تشاهد في النواس الفوضوي هي ظاهرة جديدة تنتمي الي عالم الفوضي . التحول الي الفوضي يحدث بالضبط لما $\mathcal{N} \longrightarrow \infty$ .
من اجل الحركة ذات الدور $\mathcal{N}$ نتوقع ان توجد $\mathcal{N}$ قيمة مختلفة للزاوية $\theta$ من اجل كل قيمة ل $F_D$ . الدالة $\theta$ بدلالة $F_D$ تسمي مخطط انشطار (bifurcation) و هو منحني ذو بنية منكسرة (fractal) في المنطقة الفوضوية. من هذا المخطط يمكن حساب متي يحدث بالضبط التحول نحو الفوضي.

(1) نأخذ القيم و الشروط الابتدائية

$$l = g \ , \ 2\pi\nu_D = \frac{2}{3}s^{-1} \ , \ q = \frac{1}{2}s^{-1} \ , \ N = 3000 - 100000 \ , \ dt = 0.01s.$$

$$\theta_1 = 0.2 \text{ radian} \ , \ \Omega_1 = 0 \text{ radian}/s.$$

عين دور الحركة من اجل القيم

$$F_D = 1.35 \text{ radian}/s^2 \ , \ F_D = 1.44 \text{ radian}/s^2 \ , \ F_D = 1.465 \text{ radian}/s^2.$$

ماذا يحدث للدور عندما نزيد في قيمة $F_D$. هل القيمتان الثانيتان ل $F_D$ تقعان في المنطقة الخطية ام في المنطقة الفوضوية للهزاز الفوضوي.

(2) احسب الزاوية $\theta$ بدلالة $F_D$ من اجل الازمنة التي تحقق الشرط $2\pi\nu_D t = 2n\pi$. نأخذ $F_D$ في المجال

$$F_D = (1.34 + 0.005k) \text{ radian}/s^2 \ , \ k = 1, ..., 30.$$

عين مجال قوة التحريك الخارجية الذي تكون فيه المدارات تنتمي الي الحركات ذات الدور واحد، اثنان و اربعة.

في هذا السؤال من المهم جدا ازالة الحركة الابتدائية العابرة قبل البدء في قياس مخطط الانشطار. يمكن انجاز هذا الامر كالتالي. نقوم بحساب الحركة لمدة $2N$ خطوة ثم نأخذ بعين الاعتبار فقط ال $N$ خطوة الاخيرة عند حساب مقطع بوانكري من اجل كل قيمة ل $F_D$ .

# النواس الفوضوي 4: مخططات الانشطار و الانكسار التلقائي للتناظر

الهزاز الفوضوي يعطي بمعادلة الحركة

$$\frac{d^2\theta}{dt^2} = -\sin\theta - \frac{1}{Q}\frac{d\theta}{dt} + F_D\cos 2\pi\nu_D t.$$

نأخذ عبر كل هذه المحاكاة القيم التالية

$$F_D = 1.5\ \text{radian}/s^2\ ,\ 2\pi\nu_D = \frac{2}{3}s^{-1}.$$

من اجل تحري دقة عددية اعلي نستخدم هذه المرة خوارزمية رونج - كوتا:

$$k_1 = \Delta t\ \Omega(i).$$

$$k_3 = \Delta t\ \bigg[-\sin\theta(i) - \frac{1}{Q}\Omega(i) + F_D\cos 2\pi\nu_D\Delta t(i-1)\bigg].$$

$$k_2 = \Delta t\ \bigg(\Omega(i) + \frac{1}{2}k_3\bigg).$$

$$k_4 = \Delta t\ \bigg[-\sin\bigg(\theta(i) + \frac{1}{2}k_1\bigg) - \frac{1}{Q}\bigg(\Omega(i) + \frac{1}{2}k_3\bigg) + F_D\cos 2\pi\nu_D\Delta t(i-\frac{1}{2}).\bigg].$$

$$\theta(i+1) = \theta(i) + k_2.$$

$$\Omega(i+1) = \Omega(i) + k_4.$$

$$t(i+1) = \Delta t\ i.$$

في المنطقة الخطية المدارات هي قطوع ناقصة تتميز بالتناظر

$$\theta \longrightarrow -\theta.$$

هذه المدارات بالاضافة الي كونها دورية ذات دور $T_D$ يساوي دور القوة الخارجية فهي تتميز بتناظر كامل بين اليمين و اليسار و بالتالي فان الوقت الذي يصرفه النواس في حركته الي يمين محوره الشاقولي يساوي الوقت الذي يصرفه في حركته الي يسار محوره الشاقولي.
من المثير للاهتمام وجود حلول اخري لمعادلات حركة الهزاز الفوضوي دورية ذات دور يساوي $T_D$ لكنها لا تتميز بالتناظر $\theta \longrightarrow -\theta$. في هذه الحلول نجد ان الهزاز يصرف معظم وقته اما في المنطقة $\theta < 0$ او في المنطقة $\theta > 0$ . يمكن وصف هذه الحلول غير المتناظرة بمخطط انشطار

$$\Omega = \Omega(Q).$$

من اجل كل قيمة لمعامل الجودة $Q$ فاننا نحسب مقطع بوانكري اي قيم $\theta$ و $\Omega$ في اللحظات $t = nT_D$ . نلاحظ ان مقطع بوانكري ينشطر من اجل قيمة معينة $Q_*$ ل $Q$ . تحت هذه القيمة نحصل علي خط واحد لان الحركة ذات دور $T_D$ و فوق $Q_*$ نحصل علي خطين رغم ان دورالحركة ما زال يساوي $T_D$. الخطان يقابلان الحلان اللذان يصرف فيهما الهزاز اغلب وقته في المنطقة اليمني ($\theta > 0$) او المنطقة اليسري ($\theta < 0$). الوصول الي احد الحلين انطلاقا من

**الحل المتناظر يتعلق بالشروط الابتدائية و يكون عبر زيادة قيمة $Q$ تدريجيا. هذا مثال لظاهرة الانكسار التلقائي للتناظر.**
**كما رأينا في المحاكاة السابقة يمكن ايضا وصف ظاهرة تضاعف الدور بمخطط انشطار. هذه الظاهرة هي ايضا مثال لظاهرة الانكسار التلقائي للتناظر. في هذه الحالة فان التناظر الذي ينكسر هو**

$$t \longrightarrow t + T_D.$$

**فقط الحركات التي دورها يساوي $T_D$ تتميز بهذا التناظر. لنلاحظ ان الحركات ذات الدور $\mathcal{N}$ اي المدارات التي لها دور يساوي $2^{\mathcal{N}}T_D$ لا تتميز ايضا بالتناظر $\theta \longrightarrow -\theta$.**
**لتكن $Q_{\mathcal{N}}$ قيمة $Q$ التي يحدث فيها الانشطار رقم $\mathcal{N}$ . اي ان $Q_{\mathcal{N}}$ هي القيمة التي يتحول عندها المدار من مدار ذو دور يساوي $2^{\mathcal{N}-1}T_D$ الي مدار ذو دور يساوي $2^{\mathcal{N}}T_D$. نسبة فاينباوم تعرف كالتالي**

$$F_{\mathcal{N}} = \frac{Q_{\mathcal{N}-1} - Q_{\mathcal{N}-2}}{Q_{\mathcal{N}} - Q_{\mathcal{N}-1}}.$$

**لما نقترب من المنطقة الفوضوية اي لما $\mathcal{N} \longrightarrow \infty$ فان $F_{\mathcal{N}}$ يقترب بسرعة من القيمة الثابتة**

$$F = 4.669.$$

**هذه النتيجة عامة لا تختص بالهزاز الفوضوي دون غيره من الجمل الفوضوية. في اي جملة ديناميكية يمكنها ان تتحول الي الفوضي عبر سلسلة غير منتهية من الانشطارات المرفقة بتضاعف للدور فان ثابت فاينباوم يقترب من نفس القيمة 4.669 لما $\mathcal{N} \longrightarrow \infty$ .**

(1) **اعد كتابة الشفرة باستخدام رونج - كوتا.**

(2) **نأخذ مجموعتين مختلفتين من الشروط الابتدائية**

$$\theta = 0.0 \text{ radian}\ ,\ \Omega = 0.0 \text{ radian}/s.$$

$$\theta = 0.0 \text{ radian}\ ,\ \Omega = -3.0 \text{ radian}/s\ .$$

**ادرس طبيعة المدار من اجل القيم**

$$Q = 0.5s\ ,\ Q = 1.24s\ ,\ Q = 1.3s.$$

**ماذا تلاحظ.**

**احسب مقطع بوانكري من اجل قيم $Q$ في المجال**

$$[1.2, 1.3].$$

**ارسم مخطط الانشطار $\Omega = \Omega(Q)$. ماهي القيمة $Q_*$ التي ينكسر فيها التناظر $\theta \longrightarrow -\theta$ تلقائيا.**

(3) **احسب المدار و مقطع بوانكري من اجل**

$$Q = 1.36s.$$

**ماهو دور الحركة. هل المدار متناظر تحت تأثير** $t \longrightarrow t + T_D$. **هل المدار متناظر تحت تأثير** $\theta \longrightarrow -\theta$. **ارسم مخطط الانشطار** $\Omega = \Omega(Q)$ **من اجل مجموعتين مختلفتين من الشروط الابتدائية.**

**ماهي القيمة** $Q_1$ **التي يتضاعف فيها الدور اي القيمة التي ينكسر فيها التناظر** $t \longrightarrow t + T_D$ .

(4) **في هذا السؤال و الذي يليه نستخدم الشروط الابتدائية**

$$\theta = 0.0 \text{ radian} \ , \ \Omega = 0.0 \text{ radian}/s.$$

**احسب المدار و مقطع بوانكري و ارسم مخطط الانشطار** $\Omega = \Omega(Q)$ **من اجل قيم** $Q$ **في المجال**

$$[1.34, 1.38].$$

**عين من مخطط الانشطارالقيم** $Q_{\mathcal{N}}$ **من اجل** $\mathcal{N} = 1, 2, 3, 4, 5$. **احسب ثابت فاينباوم و نقطة التراكم** $Q_\infty$ **التي يحدث عندها التحول نحو الفوضي.**

(5) **حتي نفهم التحول نحو الفوضي بطريقة افضل نعتبر هزازان فوضويان مختلفان اختلافا طفيفا. مثلا نأخذ**

$$\Delta\theta = 10^{-6} \text{ radian} \ , \ \Delta\Omega = 10^{-6} \text{ radian}/s.$$

**احسب المدار و مقطع بوانكري و عين الدور و كذلك احسب** $\ln|\Delta\Omega|$ **من اجل قيم** $Q$ **التالية**

$$Q = 1.372s \ , \ 1.375s \ , \ 1.3757s \ , \ 1.376s.$$

**ماذا تلاحظ لما نقترب من منطقة الفوضي.**

# الديناميك الجزيئي 1: توزيع ماكسويل

نعتبر حركة $N$ ذرة ارغون في بعدين داخل علبة مساحتها $L^2$. طاقة التفاعل بين اي ذرتين مفصولتين بمسافة $r$ تعطي بكمون لينارد-جونز $u$ المعرف ب

$$u = 4\epsilon\Big[\Big(\frac{\sigma}{r}\Big)^{12} - \Big(\frac{\sigma}{r}\Big)^{6}\Big].$$

القوة التي تطبقها الذرة $k$ علي الذرة $i$ هي

$$f_{k,i} = \frac{24\epsilon}{r_{ki}}\Big[2\Big(\frac{\sigma}{r_{ki}}\Big)^{12} - \Big(\frac{\sigma}{r_{ki}}\Big)^{6}\Big].$$

معادلات حركة الذرة $i$ تعطي ب

$$\frac{d^2x_i}{dt^2} = a_{x,i} = \frac{1}{m}\sum_{k\neq i} f_{k,i}\frac{x_i - x_k}{r_{ki}}\ ,\ \frac{d^2y_i}{dt^2} = a_{y,i} = \frac{1}{m}\sum_{k\neq i} f_{k,i}\frac{y_i - y_k}{r_{ki}}.$$

الخوارزمية العددية التي سنستعملها لحل هذه المعادلات التفاضلية هي خوارزمية ڤيرلات التي تعطي بالمعادلات

$$x_{i,n+1} = 2x_{i,n} - x_{i,n-1} + (\Delta t)^2 a_{x,i,n}\ ,\ y_{i,n+1} = 2y_{i,n} - y_{i,n-1} + (\Delta t)^2 a_{y,i,n}.$$

سنحسب ايضا السرعات باستعمال المعادلات التالية

$$v_{x,i,n} = \frac{x_{i,n+1} - x_{i,n-1}}{2\Delta t}\ ,\ v_{y,i,n} = \frac{y_{i,n+1} - y_{i,n-1}}{2\Delta t}.$$

من اجل التبسيط نستخدم الوحدات المختزلة $\sigma = \epsilon = m = 1$. ايضا من اجل التقليل من اثار الحواف نسعمل الشروط الحدية الدورية. اي نعتبر العلبة التي تحتوي علي الغاز علي انها تورص بدون حواف و بالتالي فانه عندما تصطدم ذرة ارغون بجدران العلبة في اي اتجاه فاننا نزيد او ننقص طول العلبة في ذلك الاتجاه كما يلي

$$\text{if } (x_i > L) \text{ then } x_i = x_i - L\ \ ,\ \ \text{if } (x_i < 0) \text{ then } x_i = x_i + L$$
$$\text{if } (y_i > L) \text{ then } y_i = y_i - L\ \ ,\ \ \text{if } (y_i < 0) \text{ then } y_i = y_i + L.$$

بسبب الشروط الحدية الدورية فان ألمسافة العظمي في الاتجاه $x$ بين اي ذرتين هو فقط $L/2$ و كذلك المسافة العظمي في الاتجاه $y$ بين اي ذرتين هو $L/2$. يتم تنفيذ هذا الامر كالتالي

$$\text{if } (x_{ij} > L/2) \text{ then } x_{ij} = x_{ij} - L\ \ ,\ \ \text{if } (x_{ij} < -L/2) \text{ then } x_{ij} = x_{ij} + L$$
$$\text{if } (y_{ij} > L/2) \text{ then } y_{ij} = y_{ij} - L\ \ ,\ \ \text{if } (y_{ij} < -L/2) \text{ then } y_{ij} = y_{ij} + L.$$

في هذه المسألة نأخذ $L$ فردي و $N$ مربع تام. الشبكة تتميز بطول الخطوة

$$a = \frac{L}{\sqrt{N}}.$$

اذن الشبكة تتشكل من $N$ خلية مساحة كل منها هي $a^2$. نختار $L$ و $N$ بحيث $a > 2\sigma$.
نختار مواضع الذرات كالتالي. الذرة $k = \sqrt{N}(i-1)+j$ توضع في مركز الخلية ذات الاركان $(i,j)$، $(i+1,j)$، $(i,j+1)$ و $(i+1,j+1)$. نقوم بعد ذلك بادخال اضطراب عشوائي علي هذه الوضعيات الابتدائية عن طريق اضافة اعداد عشوائية في المجال $[-a/4,+a/4]$ الي احداثيات الذرات. نختار السرعات الابتدائية في اتجاهات عشوائية لكن بطويلة تساوي $v_0$ من اجل جميع الذرات.

(1) اكتب شفرة ديناميك جزيئي باتباع الخطوات اعلاه. خذ $L = 15$، $N = 25$، $\Delta t = 0.02$، $\mathrm{Time} = 500$ و $v_0 = 1$. كاختبار اولي تحقق من ان الطاقة الكلية للجملة منحفظة. ارسم مسارات الجسيمات. ماذا تلاحظ.

(2) كاختبار ثاني نقترح قياس درجة الحرارة عن طريق ملاحظة كيفية اقتراب الغاز من التوازن. استعمل نظرية التقسيم المتساوي للطاقة التي تعطي ب

$$k_BT = \frac{m}{2N}\sum_{i=1}^{N}(v_{i,x}^2 + v_{i,y}^2).$$

ارسم $T$ كدالة في الزمن. خذ $\mathrm{Time} = 1000 - 1500$. ماهي درجة حرارة الغاز عند التوازن.

(3) احسب توزيع سرعات ذرات الارغون عن طريق انشاء هيستوغرام السرعات. نأخذ القيمة $\mathrm{Time} = 2000$. نعتبر سرعات كل الجسيمات في كل اللحظات. هناك $\mathrm{Time}.N$ قيمة للسرعة في هذه العينة. ننشئ هيستوغرام هذه العينة عن طريق:

- ايجاد القيمة العظمي و القيمة الصغري.
- تقسيم المجال الي سلات.
- تحديد عدد المرات التي تقع فيها قيمة معينة للسرعة داخل سلة معينة.
- تنظيم التوزيع.

قارن مع توزيع ماكسويل

$$P_{\mathrm{Maxwell}}(v) = C\frac{v^2}{k_BT}\,e^{-\frac{mv^2}{2k_BT}}.$$

استنتج درجة الحرارة من القيمة العظمي للتوزيع التي تعطي ب

$$k_BT = mv_{\mathrm{peak}}^2.$$

قارن مع درجة الحرارة المحصل عليها من نظرية التقسيم المتساوي للطاقة. ماذا يحدث اذا زدنا السرعة الابتدائية.

# الديناميك الجزيئي 2: الانصهار

نريد في هذه المسألة دراسة الانصهار الذي هو التحول الطوري من الحالة الصلبة الي الحالة السائلة. علينا اولا ان نحدد الشروط الصحيحة للحالة الصلبة. من الواضح ان درجة الحرارة يجب ان تكون منخفضة بما فيه الكفاية و الكثافة مرتفعة بما فيه الكفاية حتي تكون الحالة صلبة. من اجل خفض درجة الحرارة الي اقصي حد ممكن نبدأ من الحالة التي تكون فيها جميع الجسيمات في حالة سكون. من اجل الحصول علي تجاذب اعظمي بين الذرات نختار كثافة مساوية لجسيم واحد في كل وحدة مساحة مختزلة. نختار بالخصوص $N=16$ و $L=4$.

(1) بين انه باستعمال الشروط الابتدائية المذكورة اعلاه فاننا نحصل علي حالة صلبة بلورية ذات شبكة مثلثية.

(2) من اجل مشاهدة الانصهار يجب تسخين الجملة عن طريق زيادة الطاقة الحركية للذرات يدويا. يمكننا تحقيق هذا الامر مثلا عن طريق تغيير مواضع الجسيمات كل 1000 خطوة كالتالي

$$
\begin{aligned}
&\text{hh} = \text{int}(n/1000)\\
&\text{if } (\text{hh} * 1000.\text{eq}.n) \text{ then}\\
&x(i,n) = x(i,n+1) - R(x(i,n+1) - x(i,n))\\
&y(i,n) = y(i,n+1) - R(y(i,n+1) - y(i,n))\\
&\text{endif.}
\end{aligned}
$$

هذه العملية تؤدي الي ضرب السرعات بالقيمة $R$. نختار $R=1.5$.

تحقق من اننا نحصل بالفعل علي الانصهار بهذه الطريقة. ماذا يحدث للطاقة و درجة الحرارة.

# الاعداد العشوائية

**الجزء الاول** نعتبر مولد اعداد شبه عشوائية يعتمد علي طريقة المتبقيات المتمثلة في العلاقة

$$r_{i+1} = \text{remainder}\left(\frac{ar_i + c}{M}\right).$$

الثوابت $a$، $c$ و $M$ هم الضارب، المضاف و الطويلة علي التوالي. العدد العشوائي الابتدائي $r_i$ يسمي البذرة. نعطي القيم

$$a = 899, c = 0, M = 32768, r_1 = 12 \ \ \text{"good"}$$
$$a = 57, c = 1, M = 256, r_1 = 10\ , \ \text{"bad"}.$$

الدالة remainder تنفذ في الفورترن كالتالي

$$\text{remainder}\ \frac{a}{b} = \text{mod}(a, b).$$

(1) احسب سلسلة الاعداد العشوائية باستعمال القيم اعلاه. ارسم $r_i$ بدلالة $i$. انشئ مخطط التناثر $(x_i = r_{2i}, y_i = r_{2i+1})$.

(2) احسب متوسط الاعداد العشوائية. ماذا تلاحظ.

(3) ليكن $N$ عدد الاعداد العشوائية المولدة. احسب دوال الربط

$$\text{sum}_1(k) = \frac{1}{N-k}\sum_{i=1}^{N-k} x_i x_{i+k}\ ,\ \text{sum}_2 = \frac{\text{sum}_1(k) - < x_i >^2}{\text{sum}_1(0) - < x_i >^2}.$$

ماهو تصرف هذه الدوال في $k$.

(4) احسب دور المولدات العشوائية اعلاه.

**الجزء الثاني** نأخذ $N$ عدد عشوائي في المجال $[0, 1]$ الذي نقسمه الي $K$ مجال صغير او سلة طول كل واحدة هو $\delta = 1/K$. ليكن $N_i$ عدد الاعداد العشوائية التي تقع في السلة $i$. من اجل سلسلة اعداد عشوائية منتظمة عدد الاعداد العشوائية المتوقع في كل سلة هو $n_{\text{ideal}} = N/K$. تعرف احصائية $\chi^2-$ كالتالي

$$\chi^2 = \frac{1}{n_{\text{ideal}}}\sum_i (N_i - n_{\text{ideal}})^2.$$

(1) تحقق من النتيجة $n_{\text{ideal}} = N/K$ من اجل المولد rand الذي نجده في المكتبة المعيارية للفورترن. خذ القيم $K = 10$ و $N = 1000$. ارسم $N_i$ بدلالة الموضع $x_i$ للسلة $i$.

2) عدد درجات الحرية هو $\nu = K - 1$. القيمة الاكثر احتمالا ل $\chi^2$ هي $\nu$. تحقق من هذه النتيجة من اجل عدد كلي من اختبارات السلة يساوي $L = 1000$ و $K = 11$. في كل مرة احسب عدد المرات $L_i$ من بين ال $L = 1000$ اختبار سلة التي نحصل فيها علي قيمة معينة ل $\chi^2$. ارسم $L_i$ بدلالة $\chi^2$. ماذا تلاحظ.

# المشاء العشوائي

**الجزء الاول** نعتبر حركة مشاء عشوائي في بعد واحد. المشاء يمكنه الحركة الي اليمين خطوة تساوي $s_i = a$ باحتمال $p$ او الي اليسار خطوة تساوي $s_i = -a$ باحتمال $q = 1 - p$. بعد $N$ خطوة موضع المشاء يصبح $x_N = \sum_i s_i$ . نأخذ القيم

$$p = q = \frac{1}{2} \ , \ a = 1.$$

من اجل محاكاة حركة المشاء العشوائي نحتاج الي مولد للاعداد العشوائية. في هذه المسألة نستخدم المولد rand الذي نجده في المكتبة المعيارية للفورترن. نستدعي هذا المولد عن طريق اصدار الامر التالي

```
call srand(seed)
rand()
```

يمكن ان نستنسخ حركة المشاء العشوائي بالشفرة التالية

```
if (rand() < p) then
x_N = x_N + a
else
x_N = x_N - a
endif.
```

(1) احسب المواضع $x_i$ لثلاث مشاءات عشوائية بدلالة رقم الخطوة $i$. نأخذ $i = 1, 100$. ارسم المسارات الثلاثة.

(2) نعتبر الان حركة $K$ مشاء عشوائي حيث $K = 500$. احسب المتوسطات

$$< x_N >= \frac{1}{K}\sum_{i=1}^{K} x_N^{(i)} \ , \ < x_N^2 >= \frac{1}{K}\sum_{i=1}^{K}(x_N^{(i)})^2.$$

في المعادلات اعلاه $x_N^{(i)}$ هو موضع المشاء العشوائي $i$ بعد $N$ خطوة. ادرس تصرف هذه المتوسطات كدوال في $N$. قارن مع الحسابات النظرية.

**الجزء الثاني** نعتبر الان مشاء عشوائي في بعدين علي شبكة نقاط غير منتهية. انطلاقا من اي نقطة $(i, j)$ علي الشبكة يمكن للمشاء الوصول الي اي نقطة من نقاط الجوار الاقرب الاربعة $(i+1, j)$، $(i-1, j)$، $(i, j+1)$ و $(i, j-1)$ باحتمالات $p_x$، $q_x$، $p_y$ و $q_y$ علي التوالي حيث $p_x + q_x + p_y + q_y = 1$. من اجل التبسيط نفترض ان $p_x = q_x = p_y = q_y = 0.25$.

(1) احسب المتوسطات $< \vec{r}_N >$ و $< \vec{r}_N^2 >$ كدوال في عدد الخطوات $N$ من اجل $L = 500$ مشاء عشوائي. نعتبر القيم $N = 10, ..., 1000$.

# تقريبات النقطة الوسطي و مونتي كارلو

**الجزء الاول** يعطي حجم كرة نصف قطرها $R$ في $d$ بعد بالعلاقة

$$\begin{aligned} V_d &= \int_{x_1^2+...+x_d^2\leq R^2} dx_1...dx_d \\ &= 2\int dx_1...dx_{d-1}\sqrt{R^2-x_1^2-...-x_{d-1}^2} \\ &= \frac{R^d}{d}\frac{2\pi^{\frac{d}{2}}}{\Gamma(\frac{d}{2})}. \end{aligned}$$

(1) اكتب برنامج يحسب التكامل اعلاه في ثلاث ابعاد باستعمال طريقة النقطة الوسطي. نأخذ طول الخطوة $h=2R/N$، نصف القطر $R=1$ و عدد الخطوات في كل اتجاه يساوي $N=N_x=N_y=2^p$ حيث $p=1,15$.

(2) بين ان الخطأ يتصرف مثل $1/N$. ارسم لوغاريتم القيمة المطلقة للخطأ المطلق بدلالة لوغاريتم $N$.

(3) جرب حساب التكامل في بعدين. استعمل فقط الربع الموجب للمستوي الحقيقي و خذ طول الخطوة $h=R/N$ حيث $R=1$ و $N=2^p$، $p=1,15$. نعلم من النظري ان الخطأ يجب ان يتصرف مثل $1/N^2$. ماهو الخطأ في هذه الحالة و لماذا الاختلاف.
ملحوظة: المشتقة الثانية للدالة داخل التكامل غير معرفة عند $x=R$ مما يغير تصرف الخطأ من $1/N^2$ الي $1/N^{1.5}$.

**الجزء الثاني** من اجل حساب حجم الكرة في اي بعد $d$ عدديا نستعمل علاقة التكرار

$$V_d = \frac{V_{d-1}}{R^{d-1}}\int_{-R}^{+R} dx_d\,(R^2-x_d^2)^{\frac{d-1}{2}}.$$

(1) احسب الحجوم في الابعاد $d=4,5,6,7,8,9,10,11$. قارن بالنتيجة المضبوطة المعطاة اعلاه.

**الجزء الثالث**

(1) استعمل طريقة المعاينة لمونتي كارلو المسماة طريقة الاصابة او الخطأ من اجل حساب التكاملات في الابعاد $d=2,3,4$ و $d=10$. هل استعمال طريقة مونتي كارلو هذه اسهل من استعمال طريقة النقطة الوسطي في اي بعد.

(2) استعمل طريقة القيمة الوسطي للعينة لمونتي كارلو من اجل حساب التكاملات في الابعاد $d=2,3,4$ و $d=10$. من اجل كل $d$ نجري $M$ قياس كل واحد مشكل من $N$ عينة. نعتبر $M=1,10,100,150$ و $N=2^p$ حيث $p=10,19$. تحقق من ان الخطأ المضبوط يتصرف مثل $1/\sqrt{N}$.

ملحوظة: قارن الخطأ المضبوط الذي هو معروف في هذه الحالة مع الانحراف المعياري للمتوسط $\sigma_M$ و مع $\sigma/\sqrt{N}$ حيث $\sigma$ هو الانحراف المعياري في قياس واحد. هذه الكميات الثلاثة يجب ان تكون متساوية.

### الجزء الرابع

(1) يمكن ان تعطي قيمة $\pi$ بالتكامل

$$\pi = \int_{x^2+y^2\leq R^2} dx\ dy.$$

استعمل طريقة المعاينة لمونتي كارلو (طريقة الاصابة او الخطأ) لحساب قيمة تقريبية ل $\pi$.

(2) التكامل اعلاه يمكن ايضا ان يكتب علي الشكل

$$\pi = 2\int_{-1}^{+1} dx\ \sqrt{1-x^2}.$$

استعمل طريقة القيمة الوسطي للعينة لمونتي كارلو لحساب قيمة تقريبية ل $\pi$.

# توزيعات الاحتمال غير المنتظمة

**الجزء الاول** توزيع غوس يعطي ب

$$P(x)=\frac{1}{\sqrt{2\pi\sigma^2}}\ \exp-\frac{(x-\mu)^2}{2\sigma}.$$

الوسيط $\mu$ هو المتوسط و $\sigma$ هو التفاوت اي الجذر التربيعي للانحراف المعياري. نختار $\mu=0$ و $\sigma=1$.

(1) اكتب برنامج يحسب سلسلة من الاعداد العشوائية $x$ موزعة حسب $P(x)$ باستعمال طريقة التحويل العكسي (خوارزمية بوكس و مولر) المعطاة بالمعادلات

$$x=r\cos\phi.$$

$$r^2=-2\sigma^2\ln v\ ,\ \phi=2\pi w.$$

الاعداد $v$ و $w$ هي اعداد عشوائية منتظمة في المجال $[0,1]$.

(2) ارسم هيستوغرام للاعداد العشوائية المحصل عليها في السؤال السابق باتباع الخطوات التالية:

$a$- عين مجال الاعداد العشوائية المحصل عليها في السؤال السابق.

$b$- نقسم المجال الي $u$ سلة طول كل واحدة هو $h=\text{interval}/u$. نأخذ $u=100$.

$c$- نحدد موضع كل عدد عشوائي $x$ بين السلات. كل مرة نجد فيها عدد عشوائي في سلة معينة نزيد واحد الي العداد المرفق بهذه السلة.

$d$- نرسم نسبة الاعداد العشوائية في كل سلة بدلالة الموضع $x$. نسبة الاعداد العشوائية في كل سلة تساوي عدد الاعداد العشوائيةالتي تقع في هذه السلة علي $hN$ حيث $N$ هو العدد الكلي للاعداد العشوائية. نأخذ $N=10000$.

(3) ارسم الهيستوغرام علي سلم لوغاريتمي اي ارسم $\log(\text{fraction})$ بدلالة $x^2$. اوجد الفت و قارن مع النظرية.

**الجزء الثاني**

(1) طبق طريقة الرفض و القبول لمونتي كارلو علي المسألة اعلاه.

(2) طبق طريقة فرنانداز و كريادو علي المسالة اعلاه. الخطوات هي كالتالي:

$a$- نبدأ من $N$ نقطة $x_i$ حيث $x_i=\sigma$.

$b$ ـ نختار بشكل عشوائي زوج من النقاط $(x_i, x_j)$ من السلسلة و نقوم بالتغيير

$$x_i \longrightarrow \frac{x_i + x_j}{\sqrt{2}}$$
$$x_j \longrightarrow -x_i + \sqrt{2}x_j.$$

$c$ ـ نكرر الخطوة الثانية حتي نصل الي التوازن. مثلا كرر الخطوة الثانية $M$ مرة حيث $M = 10, 100, ...$.

# خوارزمية ميتروبوليس و نموذج ايزينغ

**الجزء الاول** نعتبر $N$ سبين علي شبكة مربعة حيث $L$ هو عدد مواقع الشبكة في كل اتجاه اي ان $N=L^2$. كل سبين يمكنه ان يأخذ احدي القيمتين $s_i=+1$ (سبين علوي) او $s_i=-1$ (سبين سفلي). كل سبين يتفاعل فقط مع جيرانه الاربعة الاقرب و ايضا مع حقل مغناطيسي خارجي $H$. نموذج ايزينغ في بعدين يعطي بدالة الطاقة

$$E=-J\sum_{<ij>}s_is_j-H\sum_i s_i.$$

السبين الموجود في نقطة تقاطع الخط $i$ و العمود $j$ يمثل بعنصر المصفوفة $\phi(i,j)$. الطاقة يمكن ان تعطي اذن ب

$$\begin{aligned}E= & -\frac{J}{2}\sum_{i,j=1}^{L}\phi(i,j)\Big(\phi(i+1,j)+\phi(i-1,j)+\phi(i,j+1)+\phi(i,j-1)\Big)\\ & - H\sum_{i=1}\phi(i,j).\end{aligned}$$

نفرض الشروط الحدية الموافقة للتورص اي

$$\phi(0,j)=\phi(n,j)\ ,\ \phi(n+1,j)=\phi(1,j)\ ,\ \phi(i,0)=\phi(i,n)\ ,\ \phi(i,n+1)=\phi(i,1).$$

نفترض ايضا ان الجملة في حالة توازن حراري مع خزان حرارة ذو درجة حرارة $T$. التقلبات الحرارية للجملة تحاكي بخوارزمية ميتروبوليس.

(1) اكتب روتين جزئي يحسب الطاقة $E$ و المغنطة $M$ في التمثيلة $\phi$ لنموذج ايزينغ. المغنطة هو وسيط ترتيب الجملة و هو معرف كالتالي

$$M=\sum_i s_i=\sum_{i,j=1}\phi(i,j).$$

(2) اكتب روتين جزئي ينفذ خوارزمية ميتروبوليس لهذه الجملة. الفرق في الطاقة الناجم عن قلب السبين $\phi(i,j)$ يعطي ب

$$\Delta E=2J\phi(i,j)\big(\phi(i+1,j)+\phi(i-1,j)+\phi(i,j+1)+\phi(i,j-1)\big)+2H\sum_{i=1}\phi(i,j).$$

(3) نختار $L=10$، $H=0$، $J=1$ و $T$ $\beta=1/T$. نعتبر حالةالانطلاقة الباردة و كذلك حالة الانطلاقة الساخنة المعرفتان علي التوالي ب

$$\phi(i,j)=+1\ \ \forall\ i,j:\ \text{Cold Start}.$$

$$\phi(i,j)=\text{rand}()\ :\ \text{Hot Start}.$$

شغل خوارزمية ميتروبوليس من اجل زمن موازنة $\text{TTH}=2^6$ و ادرس تاريخ الطاقة و المغنطة من اجل درجات حرارة مختلفة. الطاقة و المغنطة تقتربان من القيم $E=0$ و $M=0$ لما $T\longrightarrow\infty$ و من القيم $E=-2JN$ و $M=+1$ لما $T\longrightarrow 0$.

(4) ضف $TTM = 2^{10}$ خطوة مونتي كارلو و احسب متوسطات الطاقة و المغنطة.

(5) احسب السعة الحرارية و الحساسية المغناطيسية لهذه الجملة المعرفان ب

$$C_v = \frac{\partial}{\partial\beta} < E >= \frac{\beta}{T}(< E^2 > - < E >^2)\ ,\ \chi = \frac{\partial}{\partial H} < M >= \beta(< M^2 > - < M >^2).$$

(6) احسب النقطة الحرجة و قارن بالنتيجة النظرية المضبوطة

$$k_B T_c = \frac{2J}{\ln(\sqrt{2}+1)}.$$

**الجزء الثاني** ضف الي الشفرة روتين جزئي اخر ينفذ طريقة المطواة من اجل اي مجموعة من القياسات. احسب الاخطاء في الطاقة، المغنطة، السعة الحرارية و الحساسية المغناطيسية لنموذج ايزينغ باستعمال طريقة المطواة.

# التغير الطوري من الرتبة الثانية الفيرومغناطيسي

**الجزء الاول** الاساس الحرج المرفق بالسعة الحرارية يعطي ب $\alpha = 0$، اي

$$\frac{C_v}{L^2} \sim (T_c - T)^{-\alpha} \;,\; \alpha = 0.$$

هذا يعني ان السعة الحرارية تتباعد لوغاريتميا عند $T = T_c$ وهذا يظهر علي شكل تزايد لقمة السعة الحرارية (القيمة الاعظمية) مع $L$ لوغاريتميا اي

$$\frac{C_v}{L^2}|_{\rm peak} \sim \log L.$$

تحقق من هذا التصرف عدديا . استخدم شبكات بين $L = 10 - 30$ و $\text{TTH} = 2^{10}$، $\text{TMC} = 2^{13}$. درجات الحرارة تؤخذ في المجال

$$T = T_c - 10^{-2}\text{step} \;,\; \text{step} = -50, 50.$$

ارسم القيمة الاعظمية ل $C_v/L^2$ بدلالة $\ln L$.

**الجزء الثاني** المغنطة بجوار لكن تحت درجة الحرارة الحرجة تتصرف كالتالي

$$\frac{< M >}{L^2} \sim (T_c - T)^{-\beta} \;,\; \beta = \frac{1}{8}.$$

نقترح دراسة المغنطة بجوار $T_c$ من اجل تعيين قيمة $\beta$ عدديا. من اجل تحقيق هذا الهدف ارسم $| < M > |$ بدلالة $T_c - T$ حيث $T$ يؤخذ في المجال

$$T = T_c - 10^{-4}\text{step} \;,\; \text{step} = 0, 5000.$$

نعتبر شبكات كبيرة بين $L = 30 - 50$ مع $\text{TTH} = \text{TMC} = 2^{10}$. نذكر ان درجة الحرارة الحرجة في نموذج ايزينغ في بعدين تعطي ب

$$k_B T_c = \frac{2J}{\ln(\sqrt{2} + 1)}.$$

**الجزء الثالث** الحساسية المغناطيسية بجوار درجة الحرارة الحرجة في نموذج ايزينغ في بعدين تتصرف كالتالي

$$\frac{\chi}{L^2} \sim |T - T_c|^{-\gamma} \;,\; \gamma = \frac{7}{4}.$$

عين $\gamma$ عدديا . استعمل $\text{TTH} = 2^{10}$، $\text{TMC} = 2^{13}$، $L = 50$ و خذ درجة الحرارة في المجالين

$$T = T_c - 5.10^{-4}\text{step} \;,\; \text{step} = 0, 100.$$

$$T = T_c - 0.05 - 4.5.10^{-3}\text{step} \;,\; \text{step} = 0, 100.$$

# دالة الربط (غرين) الثنائية

**في هذه المسألة نواصل دراسة التغير الطوري الفيرومغناطيسي. بالخصوص سوف نحسب في هذه المسالة دالة الربط (غرين) الثنائية المعرفة بالعبارة**

$$\begin{aligned} f(n) &= < s_0 s_n > \\ &= < \frac{1}{4L^2}\sum_{i,j}\phi(i,j)\bigg(\phi(i+n,j)+\phi(i-n,j)+\phi(i,j+n)+\phi(i,j-n)\bigg) > . \end{aligned}$$

(1) **تحقق ان تصرف الدالة** $f(n)$ **عند** $T=T_c$ **يعطي ب**

$$f(n) \simeq \frac{1}{n^\eta} \ , \ \eta = \frac{1}{4}.$$

(2) **تحقق ان تصرف الدالة** $f(n)$ **من اجل** $T$ **اقل من** $T_c$ **يعطي ب**

$$f(n) = < M >^2 \ .$$

(3) **تحقق ان تصرف الدالة** $f(n)$ **من اجل** $T$ **اكبر من** $T_c$ **يعطي ب**

$$f(n) \simeq a \ \frac{1}{n^\eta} e^{-\frac{n}{\xi}}.$$

**في جميع الاسئلة اعلاه نأخذ شبكات فردية اي** $L=2LL+1$ **بين** $LL=20-50$. **نعتبر ايضا القيم** $\mathrm{TTH}=2^{10}$، $\mathrm{TTC}=2^{13}$.

(4) **بالقرب من** $T_c$ **يتباعد طول الربط كالتالي**

$$\xi \simeq \frac{1}{|T-T_c|^\nu} \ , \ \nu = 1.$$

**في هذا السؤال نأخذ** $LL=20$. **نعتبر ايضا القيم** $\mathrm{TTH}=2^{10}$، $\mathrm{TTC}=2^{15}$ **و درجات الحرارة**

$$T = T_c + 0.1.\mathrm{step} \ , \ \mathrm{step} = 0, 10.$$

**لاحظ ان جيران الدليل** $i$ **الذين يبعدون عنه مسافة** $n$ **يمكن ان يعطون بالشفرة التالية**

```
do i=1,L
do n=1,LL
if (i+n.le.L)then
ipn(i,n)=i+n
else
ipn(i,n)=(i+n)-L
endif
```

```
if ((i-n).ge.1)then
imn(i,n)=i-n
else
imn(i,n)=i-n+L
endif
enddo
enddo
```

# الهستريسيس و التغير الطوري من الرتبة الاولي

في هذه المسألة نعتبر تأثير حقل مغناطيسي علي فيزياء نموذج ايزينغ. سوف نلاحظ بالخصوص تغير طوري من الرتبة الاولي بالقرب من $H = 0$ و كذلك ظاهرة هستريسيس.

(1) نحسب المغنطة و الطاقة بدلالة $H$ من اجل درجات حرارة مختلفة. تجري الموازنة من اجل القيمة الاولي للحقل المغناطيسي و بعد حساب المغنطة المتوسطة نبدأ بتغيير الحقل المغناطيسي بشكل ادياباتيكي اي بشكل بطيء جدا عبر خطوات صغيرة حتي لا نخسر موازنة الجملة. نعتبر في هذا السؤال المجال $H = -5, 5$ مع خطوات تساوي $0.25$.

- عين من اجل $T < T_c$ (مثلا $T = 0.5$ و $T = 1.5$) موقع التغير الطوري من الرتبة الاولي من نقطة لا استمرارية (النقطة التي تقفز عندها) الطاقة و المغنطة. هذا التغير الطوري يحدث عند قيمة غير منعدمة للحقل المغناطيسي بسبب الهستريسيس. القفزة التي نلاحظها في الطاقة عند موقع التغير الطوري توافق قيمة غير منعدمة لكمية الحرارة الكامنة.
- بين ان المغنطة من اجل $T > T_c$ (مثلا $T = 3$ و $T = 5$) تصبح دالة سلسة (دالة مستمرة و قابلة للاشتقاق عدد كيفي من المرات) بالقرب من $H = 0$ و هذا يعني انه لا يوجد اي فرق بين الحالات الفيرومغناطيسية $M \geq 0$ و الحالات الفيرومغناطيسية $M \leq 0$.

(2) نعيد حساب المغنطة كدالة في $H$ من اجل المجال من $-5$ الي $5$ ذهابا و ايابا. يجب ان نلاحظ حلقة هستريسيس.

- تحقق من ان نافذة الهستريسيس تضيق بزيادة درجة الحرارة او بعد تراكم عدد اكبر من خطوات مونتي كارلو.
- ماذا يحدث عند زيادة حجم الشبكة.

تشير ظاهرة الهستريسيس الي ان تصرف الجملة يتعلق بحالتها الابتدائية و تاريخها او ان الجملة عالقة في حالات شبة مستقرة.
